# Supplementary material for: Computational Homogenization of Concrete in the Cyber Size-Resolution-Discretization (SRD) Parameter Space
Source: arXiv:2103.08957 source file (2021-03-16)
Supplement: Supplementary file 1 [file appendix_Misc-to-Surplus.tex]

%\appendix
\sect{\color{black} Appendix: Surplus}
\label{sect:Misc-to-Surplus}

%---------------------------------------------------------------------------------------------------------
  
\begin{figure}[htbp]
	\centering
	\subfloat[S32 in S371]
	{\includegraphics[height=4.0cm, angle=0]{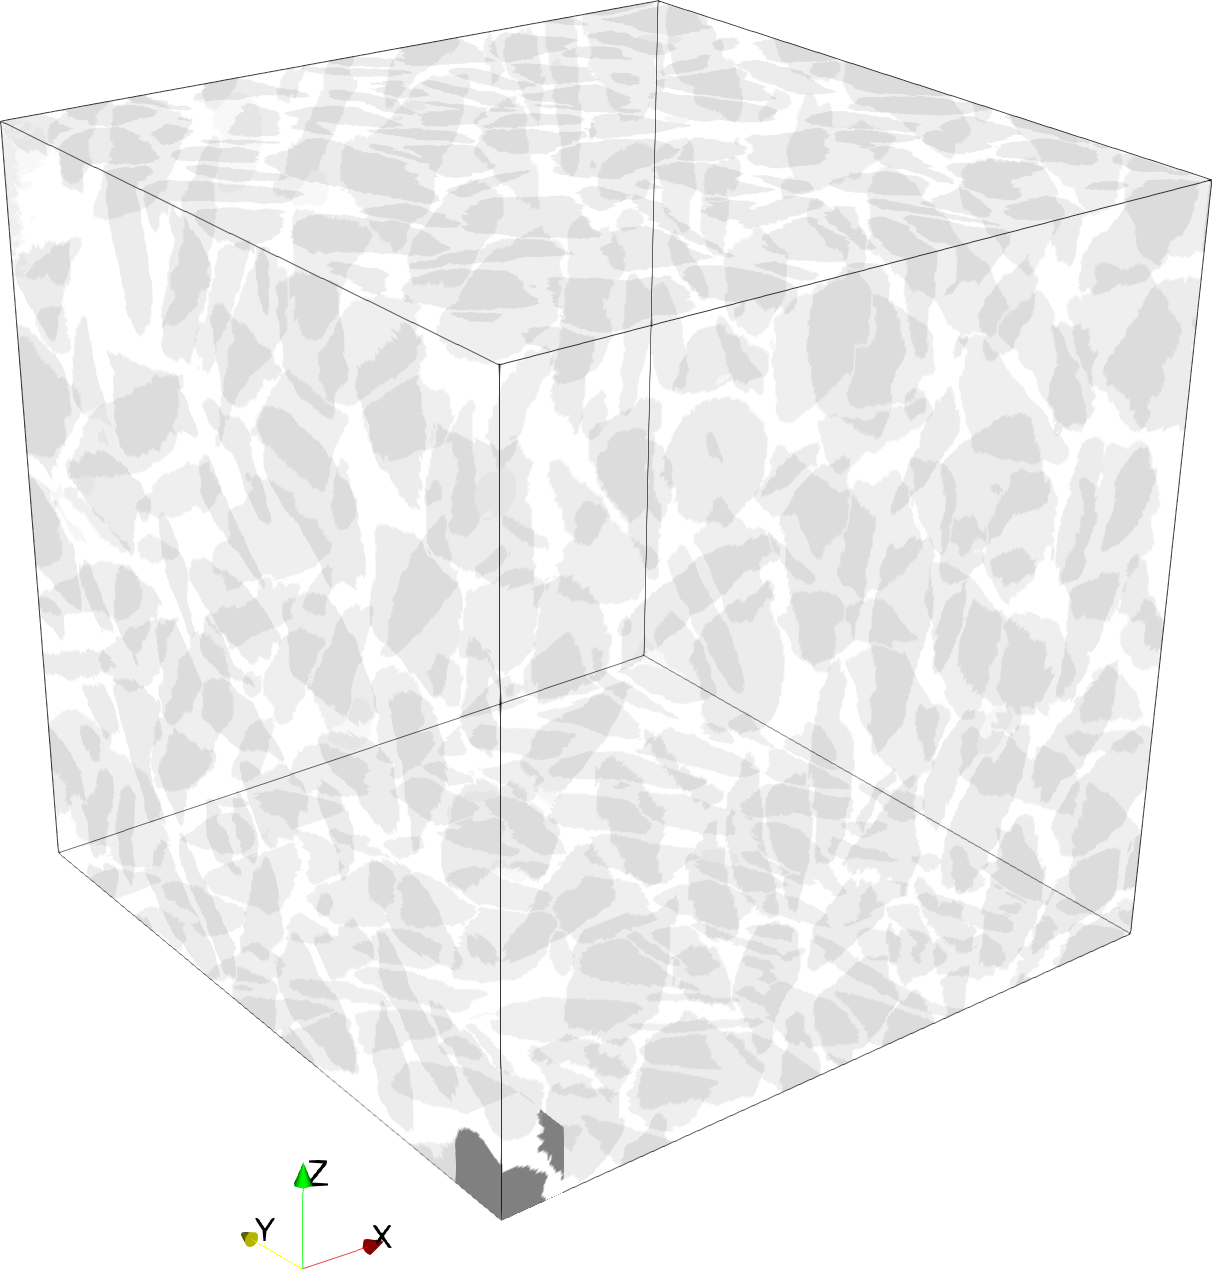}} \hspace*{0.04\linewidth}
	\subfloat[S64 in S371]
	{\includegraphics[height=4.0cm, angle=0]{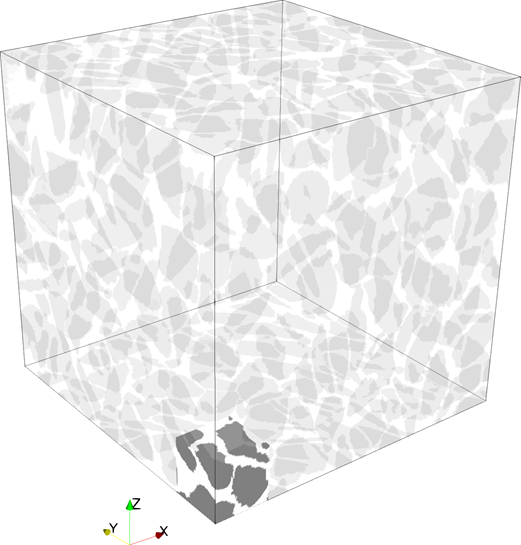}} \hspace*{0.04\linewidth}
	\subfloat[S128 in S371]
	{\includegraphics[height=4.0cm, angle=0]{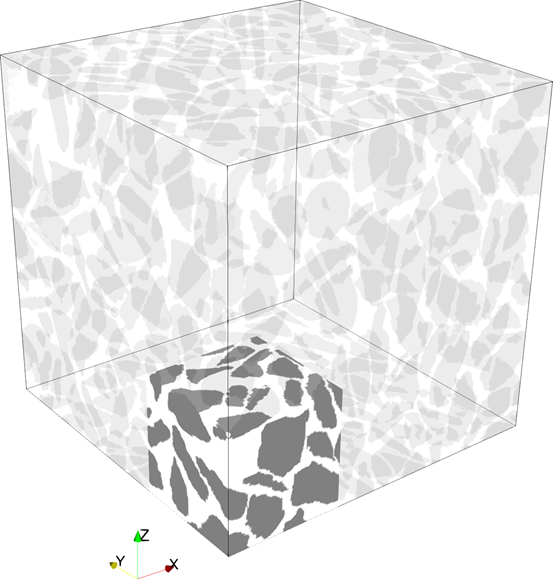}}
	\\
	\subfloat[SRD64uni]
	{\includegraphics[height=4.0cm, angle=0]{Concrete_Subvolume64_Mesh0.png}} \hspace*{0.04\linewidth}
	\subfloat[SR64-D64adap1]
	{\includegraphics[height=4.0cm, angle=0]{Concrete_Subvolume64_Mesh1.png}}
    \hspace*{0.04\linewidth}
	\subfloat[SR64-D64adap2]
	{\includegraphics[height=4.0cm, angle=0]{Concrete_Subvolume64_Mesh2.png}}
	\\
	\subfloat[SRD128uni]
	{\includegraphics[height=4.0cm, angle=0]{Concrete_Subvolume128_Mesh0.png}} \hspace*{0.04\linewidth}
	\subfloat[SR128-D128adap1]
	{\includegraphics[height=4.0cm, angle=0]{Concrete_Subvolume128_Mesh1.png}}
    \hspace*{0.04\linewidth}
	\subfloat[SR128-D128adap2]
	{\includegraphics[height=4.0cm, angle=0]{Concrete_Subvolume128_Mesh2.png}}
	\\
    \subfloat[SR320-D320adap1]
	{\includegraphics[height=4.0cm, angle=0]{Concrete_Mesh1.png}} \hspace*{0.04\linewidth}
	\subfloat[SR320-D320adap2]
	{\includegraphics[height=4.0cm, angle=0]{Concrete_Mesh2.png}}
    \hspace*{0.04\linewidth}
	\subfloat[SR320-D320adap3]
	{\includegraphics[height=4.0cm, angle=0]{Concrete_Mesh3.png}}
	\caption{\textbf{Subvolumes of different size}: (a)--(c) subvolumes with reference to full specimen size, (d)--(l) uniform and adaptively coarsened meshes.}
	\label{fig-app:Concrete_3d_meshes}
\end{figure}  

\begin{figure}[htbp]
	\centering
	\subfloat[S150 in S371]
	{\includegraphics[height=4.0cm, angle=0]{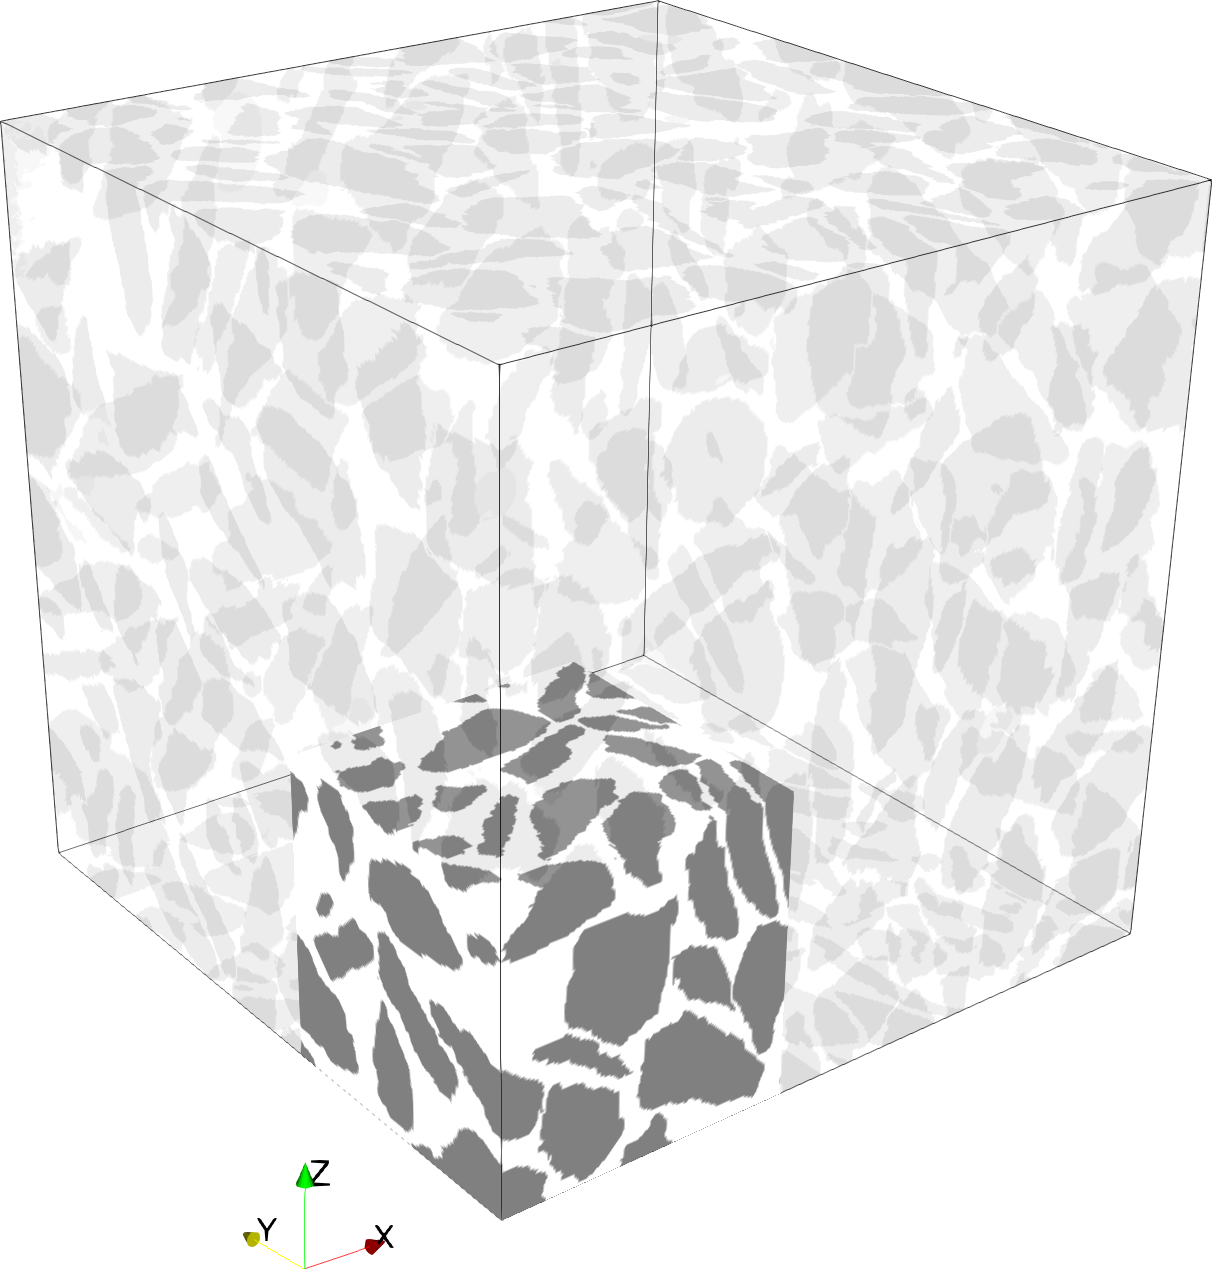}} \hspace*{0.04\linewidth}
	\subfloat[S200 in S371]
	{\includegraphics[height=4.0cm, angle=0]{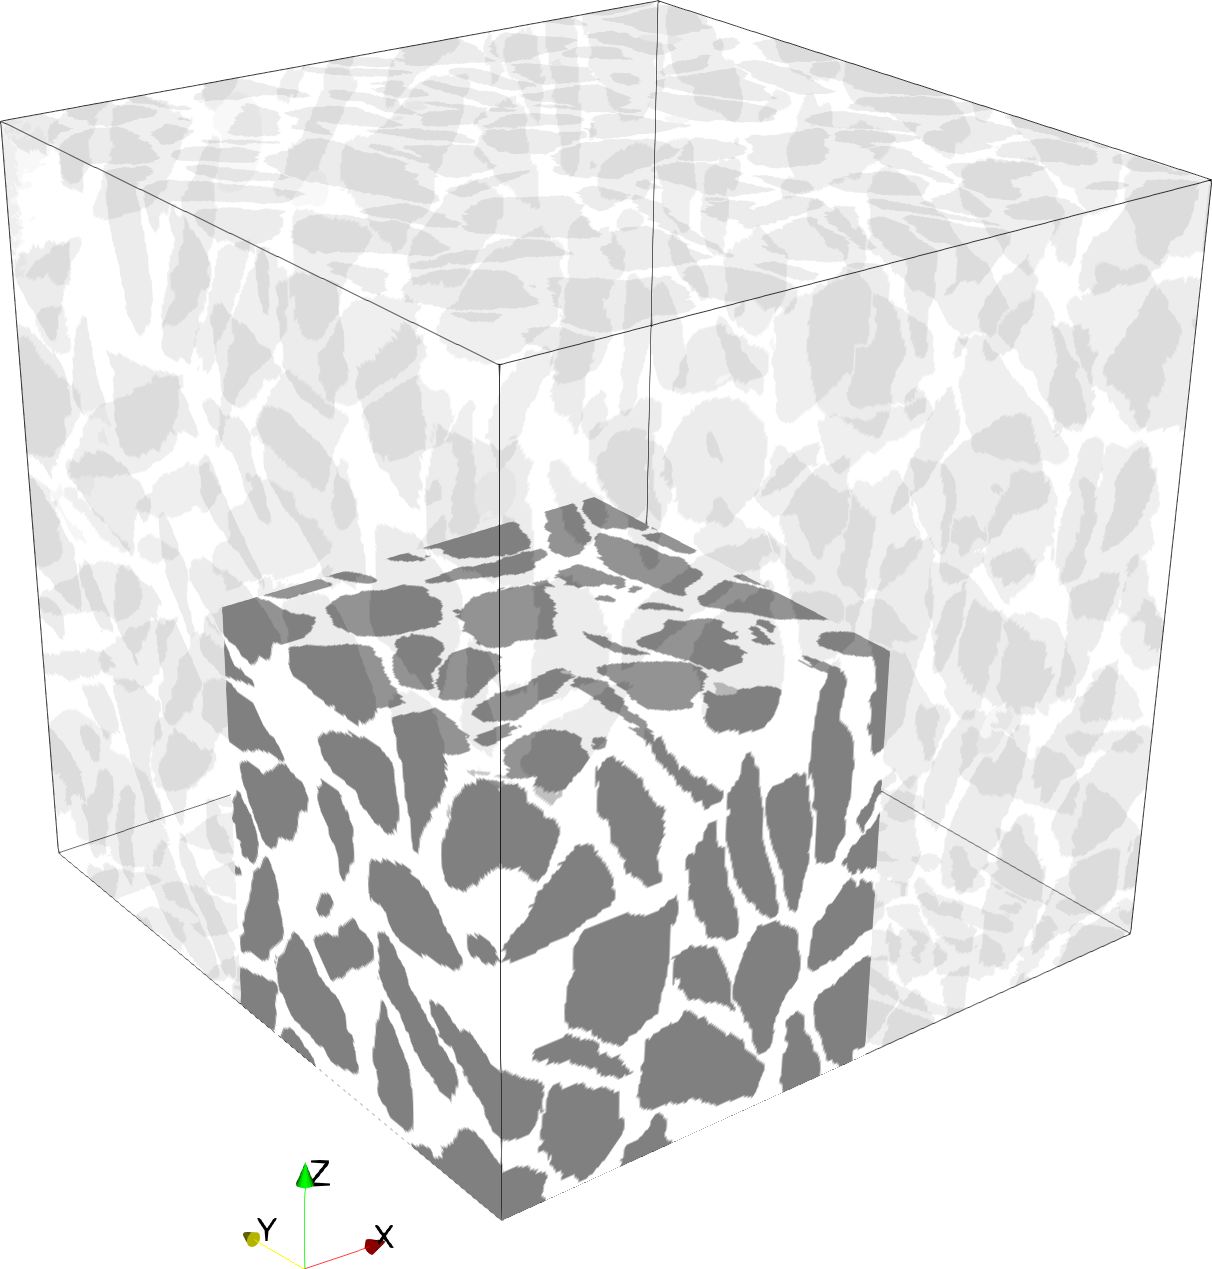}} \hspace*{0.04\linewidth}
	\subfloat[S256 in S371]
	{\includegraphics[height=4.0cm, angle=0]{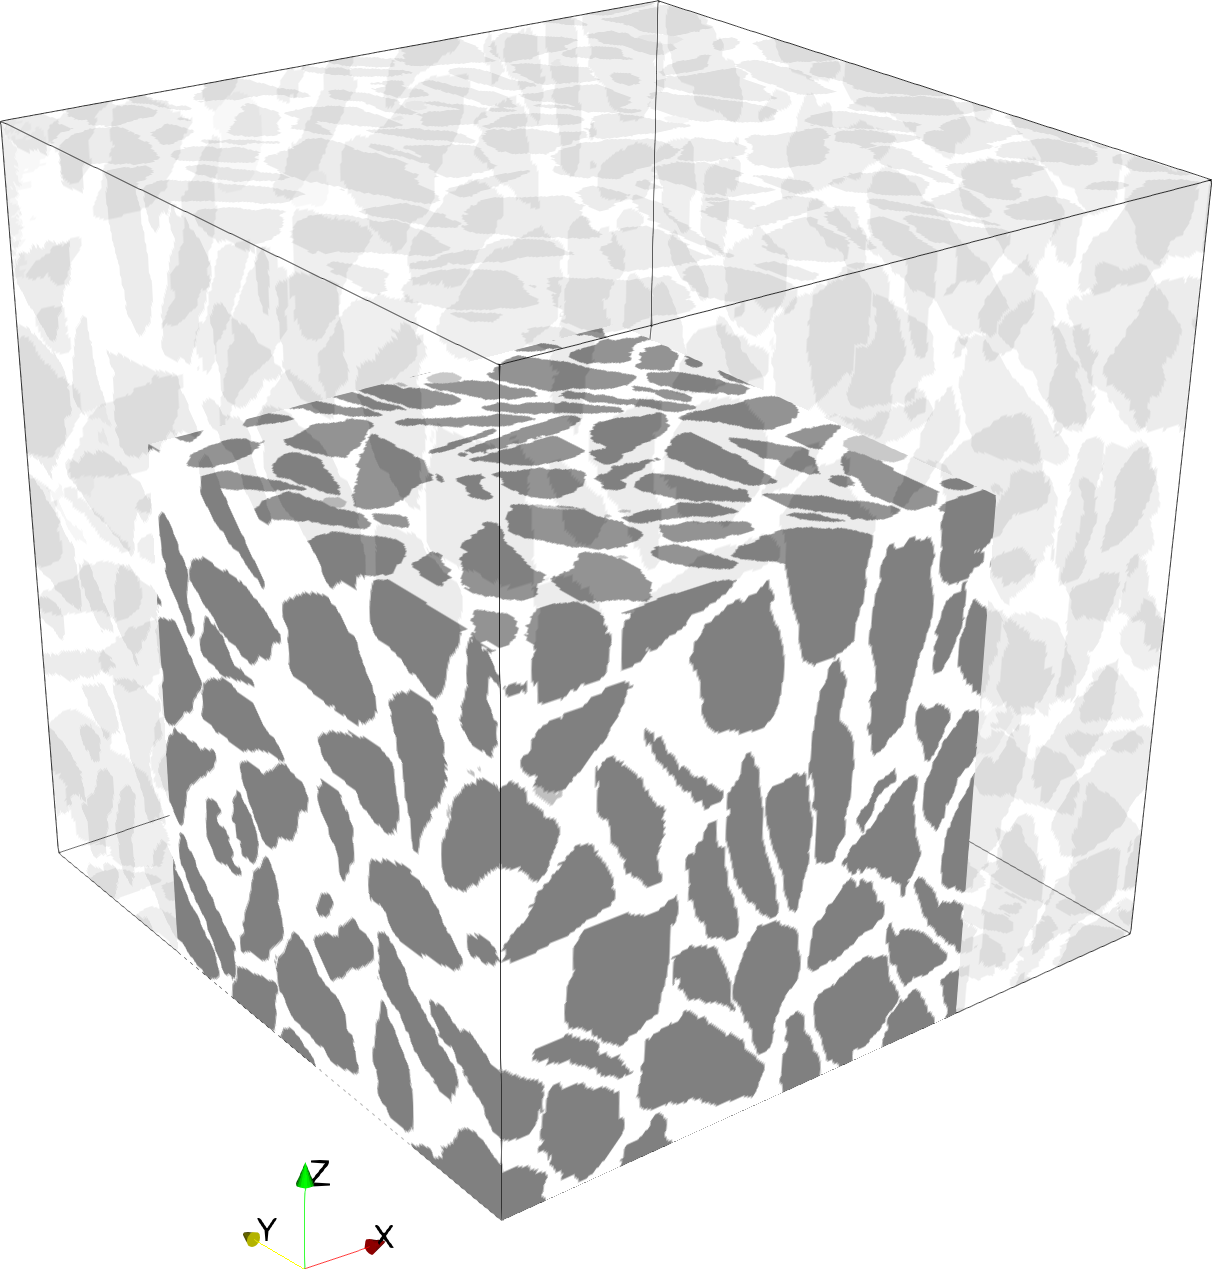}}
	\\
	\subfloat[SR256-D256adap1]
	{\includegraphics[height=4.0cm, angle=0]{Concrete_256voxel_Adap1.png}} \hspace*{0.04\linewidth}
	\subfloat[SR256-D256adap2]
	{\includegraphics[height=4.0cm, angle=0]{Concrete_256voxel_Adap2.png}} \hspace*{0.04\linewidth}
	\subfloat[SR256-D256adap3]
	{\includegraphics[height=4.0cm, angle=0]{Concrete_256voxel_Adap3.png}}
	\caption{\textbf{Subvolumes of different size}: (a) -- (c) subvolumes with reference to full specimen size, (d)--(f) octree-coarsened meshes.}
	\label{fig-app:Concrete_3d_meshes_1}
\end{figure} 

\bigskip

% ------------- error distribution

\begin{figure}[htbp]
	\centering
	\subfloat[SRD128, estimated]
	{\includegraphics[height=4.0cm, angle=0]{Estimated-Error-Concrete-128voxel-v0.png}} 
	\hspace*{0.0\linewidth}
	\subfloat[$y$-$z$ plane]
	{\includegraphics[height=4.0cm, angle=0]{Estimated-Error-Concrete-128voxel-v1.png}}
    \hspace*{0.0\linewidth}
	\subfloat[$x$-$z$ plane]
	{\includegraphics[height=4.0cm, angle=0]{Estimated-Error-Concrete-128voxel-v2.png}}
	\hspace*{0.0\linewidth}
    \subfloat[$x$-$y$ plane]
	{\includegraphics[height=4.0cm, angle=0]{Estimated-Error-Concrete-128voxel-v3.png}}	
	
	\caption{\textbf{Error distributions for SRD128:} estimated relative error distribution. }
	\label{fig-app:Concrete_3d_128vx_Estimted-Error}
\end{figure} 

\bigskip

\begin{figure}[htbp]
	\centering
	\subfloat[M256, estimated]
	{\includegraphics[height=4.0cm, angle=0]{Estimated-Error-Concrete-256voxel-256M-v0.png}} 
	\hspace*{0.0\linewidth}
	\subfloat[$y$-$z$ plane]
	{\includegraphics[height=4.0cm, angle=0]{Estimated-Error-Concrete-256voxel-256M-v1.png}}
    \hspace*{0.0\linewidth}
	\subfloat[$x$-$z$ plane]
	{\includegraphics[height=4.0cm, angle=0]{Estimated-Error-Concrete-256voxel-256M-v2.png}}
	\hspace*{0.0\linewidth}
    \subfloat[$x$-$y$ plane]
	{\includegraphics[height=4.0cm, angle=0]{Estimated-Error-Concrete-256voxel-256M-v3.png}}	
	\\
	\subfloat[M256-R128, estimated]
	{\includegraphics[height=4.0cm, angle=0]{Estimated-Error-Concrete-256voxel-128M-v0.png}}
	\hspace*{0.0\linewidth}
	\subfloat[$y$-$z$ plane]
	{\includegraphics[height=4.0cm, angle=0]{Estimated-Error-Concrete-256voxel-128M-v1.png}}
    \hspace*{0.0\linewidth}
	\subfloat[$x$-$z$ plane]
	{\includegraphics[height=4.0cm, angle=0]{Estimated-Error-Concrete-256voxel-128M-v2.png}}
	\hspace*{0.0\linewidth}
    \subfloat[$x$-$y$ plane]
	{\includegraphics[height=4.0cm, angle=0]{Estimated-Error-Concrete-256voxel-128M-v3.png}}
	\\
	\subfloat[M256-R64, estimated]
	{\includegraphics[height=4.0cm, angle=0]{Estimated-Error-Concrete-256voxel-64M-v0.png}} 
	\hspace*{0.01\linewidth}
	\subfloat[$y$-$z$ plane]
	{\includegraphics[height=4.0cm, angle=0]{Estimated-Error-Concrete-256voxel-64M-v1.png}}
    \hspace*{0.0\linewidth}
	\subfloat[$x$-$z$ plane]
	{\includegraphics[height=4.0cm, angle=0]{Estimated-Error-Concrete-256voxel-64M-v2.png}}
	\hspace*{0.0\linewidth}
    \subfloat[$x$-$y$ plane]
	{\includegraphics[height=4.0cm, angle=0]{Estimated-Error-Concrete-256voxel-64M-v3.png}}	
	\\
	\subfloat[M256-R32, estimated]
	{\includegraphics[height=4.0cm, angle=0]{Estimated-Error-Concrete-256voxel-32M-v0.png}}
	\hspace*{0.0\linewidth}
	\subfloat[$y$-$z$ plane]
	{\includegraphics[height=4.0cm, angle=0]{Estimated-Error-Concrete-256voxel-32M-v1.png}}
    \hspace*{0.0\linewidth}
	\subfloat[$x$-$z$ plane]
	{\includegraphics[height=4.0cm, angle=0]{Estimated-Error-Concrete-256voxel-32M-v2.png}}
	\hspace*{0.0\linewidth}
    \subfloat[$x$-$y$ plane]
	{\includegraphics[height=4.0cm, angle=0]{Estimated-Error-Concrete-256voxel-32M-v3.png}}
	\caption{\textbf{Error distributions in resolution coarsening:} Estimated relative error distribution for M256 and its resolution coarsened variants.}
	\label{fig-app:Concrete_3d_Estimted-Error-resolution-coarse}
\end{figure} 

\bigskip

%-------------------------------------------------------------------------------- 

\begin{figure}[htbp]
	\centering
	\subfloat[S256-R128-D128uni]
	{\includegraphics[height=4.5cm, angle=0]{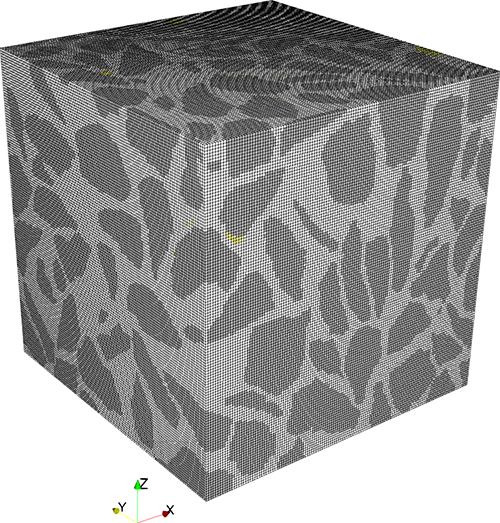}} \hspace*{0.04\linewidth}
	\subfloat[S256-R128-D128adap1]
	{\includegraphics[height=4.5cm, angle=0]{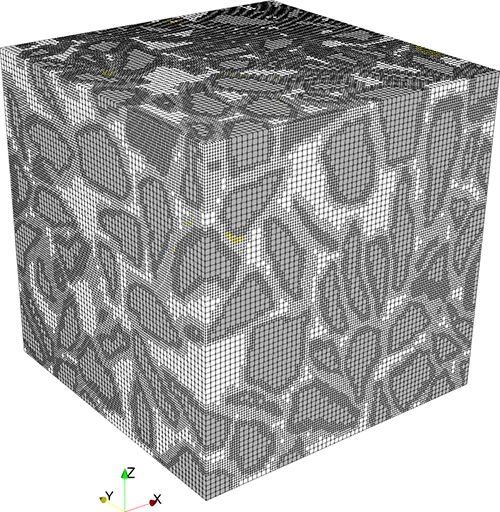}} \hspace*{0.04\linewidth}
	\subfloat[S256-R128-D128adap2]
	{\includegraphics[height=4.5cm, angle=0]{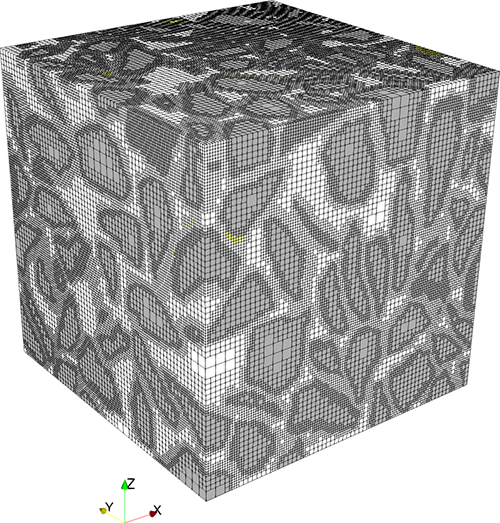}}
	\\
	\subfloat[S256-R64-D64uni]
	{\includegraphics[height=4.5cm, angle=0]{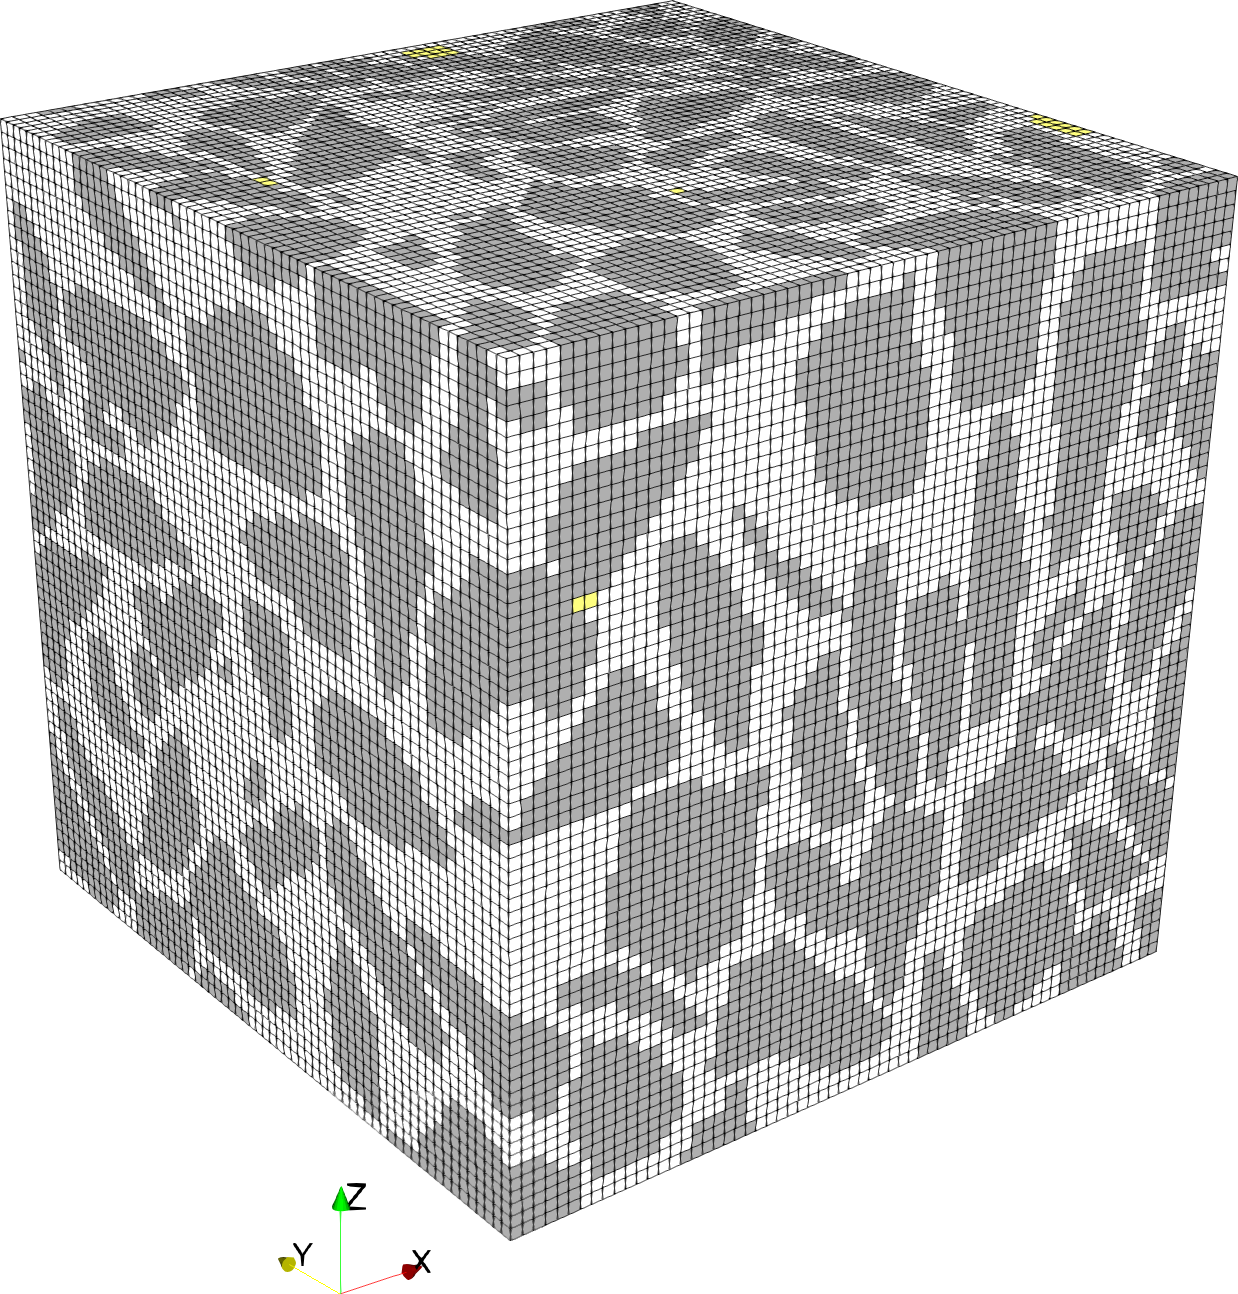}} \hspace*{0.04\linewidth}
	\subfloat[S256-R64-D64adap1]
	{\includegraphics[height=4.5cm, angle=0]{Concrete_256voxel_64meshAdp1.png}}
    \hspace*{0.04\linewidth}
	\\
	\subfloat[S256-R32-D32uni]
	{\includegraphics[height=4.5cm, angle=0]{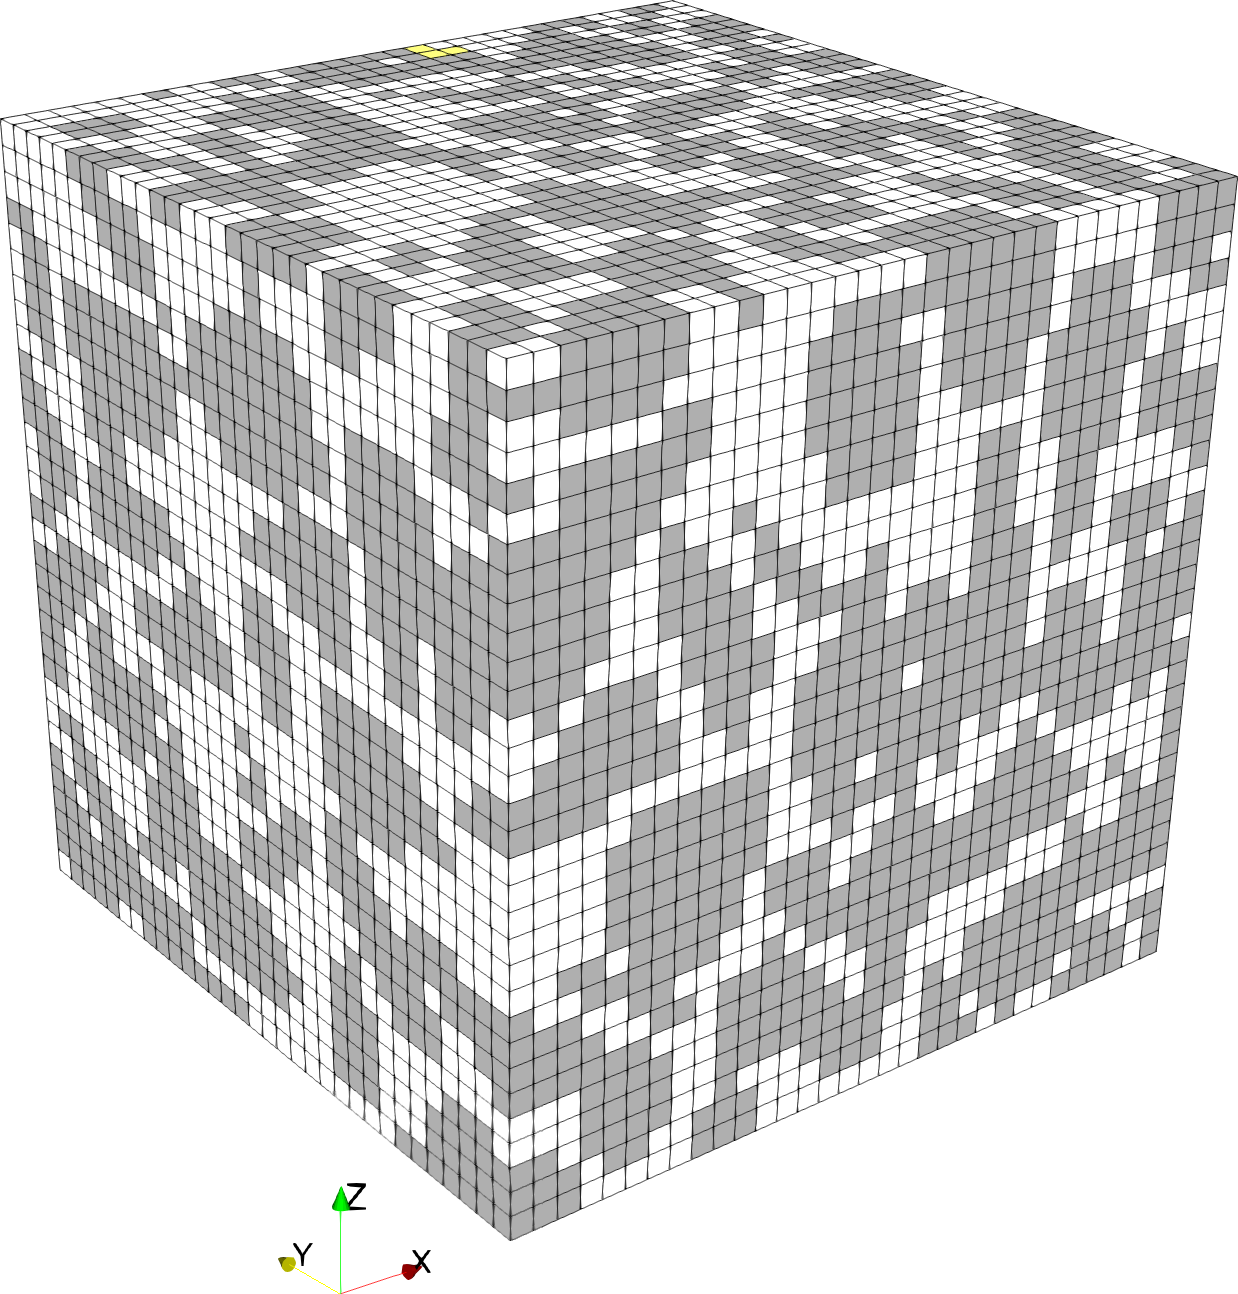}} \hspace*{0.04\linewidth}
	\subfloat[S256-R32-D32adap1]
	{\includegraphics[height=4.5cm, angle=0]{Concrete_256voxel_32meshAdp1.png}}
    \hspace*{0.04\linewidth}
	\caption{\textbf{Adaptive mesh coarsening 3d}: Adaptive mesh coarsening of the meshes obtained by resolution coarsening. {\color{red} to AG, update: adaptive mesh coarsening is not of interest here. add in the 2nd column images of the distribution of von-Mises stress, in the 3rd column the distribution of estimated errors.}}
	\label{fig-app:Concrete_3d_meshes} 
\end{figure}

%-------------------------------------------------------------------------------- 

\begin{figure}[htbp]
	\centering
%	\subfloat[S32 in S371]
%	{\includegraphics[height=4.5cm, angle=0]{Subvolume_32x32x32.png}} \hspace*{0.04\linewidth}
%	\subfloat[S64 in S371]
%	{\includegraphics[height=4.5cm, angle=0]{64outof373.png}} 
%	\hspace*{0.04\linewidth}
%	\subfloat[S128 in S371]
%	{\includegraphics[height=4.5cm, angle=0]{128outof373.png}}
%	\hspace*{0.04\linewidth}
 %   \subfloat[S256 in S371]
%	{\includegraphics[height=4.5cm, angle=0]{Subvolume_256x256x256.png}}
%	\\
	%
	\subfloat[SRD64uni]
	{\includegraphics[height=4.5cm, angle=0]{Concrete_Subvolume64_Mesh0.png}} \hspace*{0.04\linewidth}
	\subfloat[SRD64adap1]
	{\includegraphics[height=4.5cm, angle=0]{Concrete_Subvolume64_Mesh1.png}}
    \hspace*{0.04\linewidth}
	\subfloat[SRD64adap2]
	{\includegraphics[height=4.5cm, angle=0]{Concrete_Subvolume64_Mesh2.png}}
	\\
	\subfloat[SRD128uni]
	{\includegraphics[height=4.5cm, angle=0]{Concrete_Subvolume128_Mesh0.png}} \hspace*{0.04\linewidth}
	\subfloat[SRD128adap1]
	{\includegraphics[height=4.5cm, angle=0]{Concrete_Subvolume128_Mesh1.png}}
    \hspace*{0.04\linewidth}
	\subfloat[SRD128adap2]
	{\includegraphics[height=4.5cm, angle=0]{Concrete_Subvolume128_Mesh2.png}}
	\\
    \subfloat[SRD320adap1]
	{\includegraphics[height=4.5cm, angle=0]{Concrete_Mesh1.png}} \hspace*{0.04\linewidth}
	\subfloat[SRD320adap2]
	{\includegraphics[height=4.5cm, angle=0]{Concrete_Mesh2.png}}
    \hspace*{0.04\linewidth}
	\subfloat[SRD320adap3]
	{\includegraphics[height=4.5cm, angle=0]{Concrete_Mesh3.png}}
	\caption{\textbf{Subvolumes of different size}: (a)--(c) subvolumes with reference to full specimen size, (d)--(l) uniform and octree-coarsened meshes.}
	\label{fig:Concrete_3d_meshes}
\end{figure} 

Figure \ref{fig:Concrete_3d_meshes} displays in (a)--(c) some of the considered specimen sizes, in (d)--(l) selected specimens in uniform and adaptively coarsened discretizations. {\color{blue} these images are a luxury, candidates for being deleted.} 

\newpage
\begin{figure}[htbp]
	\centering
	\subfloat[SRD256, estimated]
	{\includegraphics[height=4.0cm, angle=0]{Estimated-Error-Concrete-256voxel-256M-v0.png}} 
	\hspace*{0.0\linewidth}
	\subfloat[$YZ$-plane]
	{\includegraphics[height=4.0cm, angle=0]{Estimated-Error-Concrete-256voxel-256M-v1.png}}
    \hspace*{0.0\linewidth}
	\subfloat[$XZ$-plane]
	{\includegraphics[height=4.0cm, angle=0]{Estimated-Error-Concrete-256voxel-256M-v2.png}}
	\hspace*{0.0\linewidth}
    \subfloat[$XY$-plane]
	{\includegraphics[height=4.0cm, angle=0]{Estimated-Error-Concrete-256voxel-256M-v3.png}}	
	\\
	\subfloat[SRD300, estimated]
	{\includegraphics[height=4.0cm, angle=0]{Estimated-Error-Concrete-300voxel-300M-v0.png}}
	\hspace*{0.0\linewidth}
	\subfloat[$YZ$-plane]
	{\includegraphics[height=4.0cm, angle=0]{Estimated-Error-Concrete-300voxel-300M-v1.png}}
    \hspace*{0.0\linewidth}
	\subfloat[$XZ$-plane]
	{\includegraphics[height=4.0cm, angle=0]{Estimated-Error-Concrete-300voxel-300M-v2.png}}
	\hspace*{0.0\linewidth}
    \subfloat[$XY$-plane]
	{\includegraphics[height=4.0cm, angle=0]{Estimated-Error-Concrete-300voxel-300M-v3.png}}
	\
	\subfloat[SRD320, estimated]
	{\includegraphics[height=4.0cm, angle=0]{Estimated-Error-Concrete-320voxel-320M-v0.png}} 
	\hspace*{0.01\linewidth}
	\subfloat[$YZ$-plane]
	{\includegraphics[height=4.0cm, angle=0]{Estimated-Error-Concrete-320voxel-320M-v1.png}}
    \hspace*{0.0\linewidth}
	\subfloat[$XZ$-plane]
	{\includegraphics[height=4.0cm, angle=0]{Estimated-Error-Concrete-320voxel-320M-v2.png}}
	\hspace*{0.0\linewidth}
    \subfloat[$XY$-plane]
	{\includegraphics[height=4.0cm, angle=0]{Estimated-Error-Concrete-320voxel-320M-v3.png}}	
	\\
	\subfloat[SRD371, estimated]
	{\includegraphics[height=4.0cm, angle=0]{Estimated-Error-Concrete-371voxel-371M-v0.png}}
	\hspace*{0.0\linewidth}
	\subfloat[$YZ$-plane]
	{\includegraphics[height=4.0cm, angle=0]{Estimated-Error-Concrete-371voxel-371M-v1.png}}
    \hspace*{0.0\linewidth}
	\subfloat[$XZ$-plane]
	{\includegraphics[height=4.0cm, angle=0]{Estimated-Error-Concrete-371voxel-371M-v2.png}}
	\hspace*{0.0\linewidth}
    \subfloat[$XY$-plane]
	{\includegraphics[height=4.0cm, angle=0]{Estimated-Error-Concrete-371voxel-371M-v3.png}}
	\caption{\textbf{Estimated error distributions}: Estimated relative error, for SRD256:(a)--(d), for SRD300:(e)--(h), for SRD300:(i)--(l) and for SRD371:(m)--(p).}
	\label{fig:Concrete_3d_256-371vx_Estimted-Error}
\end{figure}
