# Supplementary material for: Computational Homogenization of Concrete in the Cyber Size-Resolution-Discretization (SRD) Parameter Space
Source: arXiv:2103.08957 source file (2021-03-16)
Supplement: Supplementary file 2 [file appendix_Miscellaneous.tex]

\sect{\color{black} Appendix}
\label{sect:Miscellaneous}
%---------------------------------------------------------------------------------

%\subsection{More data to simulation results}

\begin{Table}[htbp]
%	\begin{minipage}{16.5cm}  
%		\footnotesize
		\centering
		 
 		\resizebox{0.5\columnwidth}{!}{ 
		\begin{tabular}{c c c c c c c}
\toprule
	        &   \multicolumn{5}{c}{SRD}       \\ 
            & 160    &  200   &  240    &  280   &  320  &  371   \\
\midrule
			&   \multicolumn{5}{c}{phase fractions} \\   
			aggregate            & $0.5759$	& $0.5994$ & $0.5629$ & $0.5549$ & $0.5629$ & $0.5624$ \\ 
			mortar               & $0.4186$	& $0.3970$ & $0.4347$ & $0.4433$ & $0.4357$ & $ 0.4366$ \\ 
			pore                 & $0.0055$	& $0.0036$ & $0.0025$ & $0.0018$ & $0.0014$ & $0.0010$	 \\ 
\midrule
            &   \multicolumn{6}{c}{periodic}       \\
			$\mathbb{C}_{11}$  & $36216$ & $37028$ & $35953$	& $35550$ & $35786$ & $35858$ \\ 	
			$\mathbb{C}_{22}$  & $35031$ & $36239$ & $35223$ & $35354$	&  $35631$ & $35638$ \\ 
			$\mathbb{C}_{33}$  & $13355$ & $13764$ & $13274$ & $13172$	&  $13310$& $13334$ \\ 
			$\mathbb{C}_{12}=\mathbb{C}_{21}$   & $9132$ & $9392$ & $9051$ & $8962$ & $9053$ & $9070$ \\ 
			\midrule
            &   \multicolumn{6}{c}{dirichlet}       \\
			$\mathbb{C}_{11}$  & $36494$ & $37330$ & $36222$	& $35779$ & $35999$ & $36121$ \\ 	
			$\mathbb{C}_{22}$  & $35654$ & $36688$ & $35476$	& $35507$ & $35862$ & $35993$ \\
			$\mathbb{C}_{33}$  & $13622$ & $13923$ & $13468$	& $13324$ & $13446$ & $13479$ \\
			$\mathbb{C}_{12}=\mathbb{C}_{21}$   & $9111$ & $9341$ & $9036$	& $8941$ & $9022$ & $9053$ \\
			\midrule
            &   \multicolumn{6}{c}{neumann}       \\
			$\mathbb{C}_{11}$  & $35512$ & $36716$ & $35460$	& $35261$ & $35464$ & $35621$ \\ 	
			$\mathbb{C}_{22}$  & $33159$ & $35780$ & $34903$ & $34938$	&  $35351$ & $35600$ \\ 
			$\mathbb{C}_{33}$  & $13102$ & $13607$ & $13180$ & $13089$	&  $13222$& $13280$ \\ 
			$\mathbb{C}_{12}=\mathbb{C}_{21}$   & $8667$ & $9221$ & $8960$ & $8884$ & $8972$ & $9005$ \\ 
\bottomrule
		\end{tabular} 
}
%	\end{minipage}
	\caption{\textbf{Homogenized 2d elasticity tensor:} $\mathbb{C}_{ij}$ (MPa) for different SRD and different coupling conditions.}
	\label{tab:component-elast-tensor_RAE_size} 
\end{Table}

\begin{Table}[htbp]
%	\begin{minipage}{16.5cm}  
%		\footnotesize
		\centering
		 
 		\resizebox{0.7\columnwidth}{!}{ 
		\begin{tabular}{c c c c c c c c}
\toprule
SD320       &   \multicolumn{7}{c}{resolution coarsening}       \\ 
	        & \multicolumn{3}{c}{phase averaging} & \multicolumn{3}{c}{phase preserving} & reference\\
resolution R &  40    &  80    &  160  &  40    & 80    &  160  &  320   \\
\midrule
			&   \multicolumn{7}{c}{phase fractions} \\
			aggregate            & $0.5629$	& $0.5629$ & $0.5629$ & $0.5569$ & $0.5530$ & $0.5554$ & $0.5629$	 \\ 
			mortar               & $0.4357$	& $0.4357$ & $0.4357$ & $0.4419$ & $0.4456$ & $0.4433$ & $0.4357$	 \\ 
			pore                 & $0.0014$	& $0.0014$ & $0.0014$ & $0.0013$ & $0.0014$ & $0.0013$ & $0.0014$	 \\ 
\midrule
            &   \multicolumn{6}{c}{$\mathbb{C}_{ij}$ in (MPa) }       \\
			$\mathbb{C}_{11}$  & $37814$ & $36827$ & $36196$ & $35836$ & $35545$ & $35532$ & $35786$	 \\ 	
			$\mathbb{C}_{22}$  & $37686$ & $36620$ & $36003$ & $35640$ & $35307$ & $35402$ &  $35631$ \\ 
			$\mathbb{C}_{33}$  & $14009$ & $13656$ & $13446$ & $13197$ & $13152$ & $13202$ &  $13310$ \\ 
			$\mathbb{C}_{12}=\mathbb{C}_{21}$   & $9482$ & $9271$ & $9146$ & $8987$ & $8952$ & $8983$ & $9053$ \\ 
\bottomrule
		\end{tabular} 
 }
%	\end{minipage}
	\caption{\textbf{Homogenized elasticity tensor:} components $\mathbb{C}_{ij}$ of size S320 at different resolutions R but each which discretization D320, hence S320-R\,$i$-D320.} 
	\label{tab:component-elast-tensor_resolution} 
\end{Table}

\begin{Table}[H]
%	\begin{minipage}{16.5cm}  
%		\footnotesize
		\centering
		 
 		\resizebox{0.50\columnwidth}{!}{ 
		\begin{tabular}{c c c c c}
\toprule
SR320       &   \multicolumn{4}{c}{uniform mesh refinement} \\
discretization D &  320   &  640  &   1280  &    1920  \\
\midrule
%            &   \multicolumn{4}{c}{elasticity tensor components (in MPa)}       \\
			$\mathbb{C}_{11}$  & $35786$  & $35739$ & $35723$ & $35720$ \\ 	
			$\mathbb{C}_{22}$  & $35631$  & $35582$ & $35566$ & $35562$ \\   
			$\mathbb{C}_{33}$  & $13310$  & $13292$ & $13284$ & $13283$ \\  
			$\mathbb{C}_{12}=\mathbb{C}_{21}$ & $9053$ & $9056$ & $9058$ & $9058$ \\  
\bottomrule
		\end{tabular} 
 }
%	\end{minipage}
	\caption{\textbf{Homogenized 2d elasticity tensor:} $\mathbb{C}_{ij}$ (MPa) for different discretizations.}
	\label{tab:component-elast-tensor_discretization} 
\end{Table}

%-------------------------------------------------------------------------------------------

\begin{Table}[htbp]
%	\begin{minipage}{16.5cm}  
%		\footnotesize
		\centering
		 
		\resizebox{0.8\columnwidth}{!}{%
		\begin{tabular}{c c c c c c c c c c c}
\toprule
	        &   \multicolumn{10}{c}{SRD}       \\ 
            &  16   &   32    &   64   &  128   &   150  &  200   &  256  & 300 & 320  & 371 \\
\midrule
			&   \multicolumn{10}{c}{volume fraction}       \\   
			aggregate            & 0.725	& 0.598	& 0.557	& 0.550	& 0.544	& 0.563	& 0.558 & 0.556 & 0.558 & 0.559 \\ 
			mortar               & 0.275	& 0.403	& 0.443	& 0.447	& 0.453	& 0.434	& 0.432 & 0.433 & 0.431 & 0.432 \\ 
			pore                 & 0.000	& 0.000	& 0.000	& 0.003	& 0.003	& 0.003	& 0.010 & 0.012 & 0.011 & 0.009 \\   
\midrule
            &   \multicolumn{10}{c}{elasticity tensor components (in MPa) }       \\
			$\mathbb{C}_{11}$                   & 50926	& 45489	& 44283	& 43321	& 43099	& 43659 & 42698 & 42506 & 42650 & 42856 \\
			$\mathbb{C}_{22}$                   & 52360	& 46231	& 44595	& 43642	& 43151	& 43964 & 43363 & 43132 & 43291 & 43444 \\
			$\mathbb{C}_{33}$                   & 52854	& 45713	& 43369	& 43684	& 43616	& 44291 & 43493 & 43197 & 43352 & 43576 \\
			$\mathbb{C}_{44}$                   & 15174	& 13233	& 12727	& 12728	& 12651	& 12871 & 12699 & 12625 & 12672 & 12716 \\
			$\mathbb{C}_{55}$                   & 14778	& 13543	& 12801	& 12641	& 12608	& 12778 & 12555 & 12499 & 12539 & 12602 \\
			$\mathbb{C}_{66}$                   & 14840	& 13186	& 12890	& 12673	& 12588	& 12752 & 12543 & 12483 & 12528 & 12568 \\
			$\mathbb{C}_{12}=\mathbb{C}_{21}$   & 21554	& 18985	& 18434	& 18107	& 18005	& 18241 & 17795 & 17692 & 17768 & 17865 \\
			$\mathbb{C}_{13}=\mathbb{C}_{31}$   & 21491	& 19393	& 18400	& 18084	& 18008	& 18252 & 17795 & 17691 & 17763 & 17883 \\
			$\mathbb{C}_{23}=\mathbb{C}_{32}$   & 21867	& 19007	& 18313	& 18159	& 18050	& 18327 & 17925 & 17796 & 17875 & 17972 \\
\bottomrule
		\end{tabular} 
}
%	\end{minipage}
	\caption{\textbf{Homogenized 3d elasticity tensor:} $\mathbb{C}_{ij}$ for different SRD.}
	\label{tab:component-elast-tensor} 
\end{Table}

\begin{Table}[htbp]
%	\begin{minipage}{16.5cm}  
%		\footnotesize
		\centering
		 
 		\resizebox{0.7\columnwidth}{!}{
		\begin{tabular}{c c c c c c c c}
\toprule
S256       &   \multicolumn{7}{c}{resolution coarsening}       \\ 
	        & \multicolumn{3}{c}{phase averaging} & \multicolumn{3}{c}{phase preserving} & reference\\
resolution R &  32    &  64    &  128  &  32    & 64    &  128  &  256   \\
\midrule
			&   \multicolumn{7}{c}{phase fractions} \\
			aggregate            & $0.558$	& $0.558$ & $0.558$ & $0.580$ & $0.554$ & $0.542$ & $0.558$	 \\ 
			mortar               & $0.432$	& $0.432$ & $0.432$ & $0.416$ & $0.438$ & $0.450$ & $0.432$	 \\ 
			pore                 & $0.010$	& $0.010$ & $0.010$ & $0.005$ & $0.007$ & $0.009$ & $0.010$	 \\ 
\midrule
            &   \multicolumn{7}{c}{$\mathbb{C}_{ij}$ in (MPa) }       \\
			$\mathbb{C}_{11}$                   & $46342$ & $44691$ & $43537$ & $45826$ & $43578$ & $42390$ & $42698$  \\ 	
			$\mathbb{C}_{22}$                   & $46643$ & $45162$ & $44121$ & $46164$ & $44152$ & $43032$ & $43363$ \\ 
			$\mathbb{C}_{33}$                   & $46676$ & $45269$ & $44262$ & $46283$ & $44314$ & $43187$ & $43493$ \\ 
			$\mathbb{C}_{44}$                   & $13446$ & $13112$ & $12875$ & $13374$ & $12863$ & $12576$ & $12699$   \\ 
			$\mathbb{C}_{55}$                   & $13390$ & $13016$ & $12750$ & $13299$ & $12740$ & $12436$ & $12555$   \\
			$\mathbb{C}_{66}$                   & $13378$ & $12999$ & $12735$ & $13280$ & $12718$ & $12420$ & $12543$   \\
			$\mathbb{C}_{12}=\mathbb{C}_{21}$   & $19492$ & $18708$ & $18190$ & $19001$ & $18101$ & $17649$ & $17795$   \\
			$\mathbb{C}_{13}=\mathbb{C}_{31}$   & $19502$ & $18724$ & $18200$ & $19025$ & $18125$ & $17658$ & $17795$   \\
			$\mathbb{C}_{23}=\mathbb{C}_{32}$   & $19573$ & $18824$ & $18317$ & $19109$ & $18247$ & $17786$ & $17925$   \\
			
\bottomrule
		\end{tabular}  
}
%	\end{minipage}
	\caption{\textbf{Uniform coarsening of resolution and discretization:} $\mathbb{C}_{ij}$ for S256-RD\,$i$, for phase-avaeraging and phase-preserving coarsening with element size equal to the voxel size.} 
	\label{tab:component-elast-tensor-256voxel-and-meshes} 
\end{Table}

\begin{Table}[htbp]
%	\begin{minipage}{16.5cm}  
%		\footnotesize
		\centering
		 
 		\resizebox{0.7\columnwidth}{!}{
		\begin{tabular}{c c c c c c c c}
\toprule
S256       &   \multicolumn{7}{c}{resolution coarsening}       \\ 
	        & \multicolumn{3}{c}{phase averaging} & \multicolumn{3}{c}{phase preserving} & reference\\
resolution R &  32    &  64    &  128  &  32    & 64    &  128  &  256   \\
\midrule
			&   \multicolumn{7}{c}{phase fractions} \\
			aggregate                          & $0.558$  & $0.558$ & $0.558$ & $0.580$ & $0.554$ & $0.542$ & $0.558$	\\ 
			mortar                             & $0.432$  & $0.432$ & $0.432$ & $0.416$ & $0.438$ & $0.450$ & $0.432$	\\ 
			pore                               & $0.010$  & $0.010$ & $0.010$ & $0.005$ & $0.007$ & $0.009$ & $0.010$	\\ 
\midrule
            &   \multicolumn{7}{c}{$\mathbb{C}_{ij}$ in (MPa) }       \\
			$\mathbb{C}_{11}$                   & $45951$ & $44452$ & $43421$ & $44661$ & $42966$ & $42160$ & $42698$	\\
			$\mathbb{C}_{22}$                   & $46261$ & $44920$ & $44002$ & $45013$ & $43535$ & $42796$ & $43363$	\\ 
			$\mathbb{C}_{33}$                   & $46294$ & $45031$ & $44143$ & $45158$ & $43707$ & $42950$ & $43493$	\\ 
			$\mathbb{C}_{44}$                   & $13320$ & $13029$ & $12835$ & $13036$ & $12681$ & $12508$ & $12699$	\\ 
			$\mathbb{C}_{55}$                   & $13262$ & $12934$ & $12711$ & $12959$ & $12558$ & $12369$ & $12555$	\\
			$\mathbb{C}_{66}$                   & $13252$ & $12917$ & $12696$ & $12939$ & $12537$ & $12354$ & $12543$	\\
			$\mathbb{C}_{12}=\mathbb{C}_{21}$   & $19343$ & $18621$ & $18145$ & $18538$ & $17867$ & $17556$ & $17795$	\\
			$\mathbb{C}_{13}=\mathbb{C}_{31}$   & $19347$ & $18632$ & $18153$ & $18552$ & $17883$ & $17563$ & $17795$	\\
			$\mathbb{C}_{23}=\mathbb{C}_{32}$   & $19411$ & $18726$ & $18266$ & $18626$ & $17994$ & $17685$ & $17925$	\\
			
\bottomrule
		\end{tabular}  
}
%	\end{minipage}
	\caption{\textbf{Homogenized elasticity tensor:} components $\mathbb{C}_{ij}$ of size S256 at different resolutions R but each with discretization D256, hence S256-R\,$i$-D256.} 
	\label{tab:component-elast-tensor-256voxel-RiD256} 
\end{Table}

\begin{Table}[htbp]
%	\begin{minipage}{16.5cm}  
%		\footnotesize
\centering
 
\resizebox{0.8\columnwidth}{!}{%
	\begin{tabular}{c c c c c c c c c}
	\toprule
	&   \multicolumn{8}{c}{SRD}       \\ 
	&  16   &   32    &   64   &  128   &  256  & 300 & 320  & 371 \\  
	\midrule
	&   \multicolumn{8}{c}{estimated error in energy norm (in Nmm) }       \\
	$\bar e_{\text{mic}}$               & 1.3227	& 3.6734	& 8.6605	& 26.8484	& 80.9352	& 102.4414 & 112.1215 & 138.4225 \\
	
	\bottomrule
	\end{tabular} 
}
%	\end{minipage}
\caption{\textbf{Estimated error:} estimated errors in the energy norm $\bar e_{\text{mic}}$ for SRD16, 32, 64, 128, 256, 300, 320, 371. Errors in (Nmm).}
\label{tab:estimated-error-3D-specimen} 
\end{Table}
